# Supplementary material for: Practical Data Poisoning Attack against Next-Item Recommendation
Source: arXiv:2004.03728 source file (2020-04-07)
Supplement: Supplementary file 1 [file appendix.tex]

\section{Training Algorithm of DQN}

In each iteration on a training session, there are two stages. 
For replay memory generation stage: given the state $s_t$, the agent first samples an action at according to an $\epsilon$-greedy policy, in which an action is sampled either totally randomly or from the fixed off-policy implicitly suggested by
the off-policy Q-function. The ratio of randomly sampled actions $\epsilon$, which
decreases from 1 to 0.05 to help the model get more diverse samples
during the early training state. 
Then the agent observes the reward $r_t$ from the outcome estimator and updates the state. 
For Q-network training stage: the manipulation agent samples a $(s_t, a_t, r_t, s_{t+1})$ from replay memory $D$, and then updates the parameters according to Equation:
\begin{equation}
    \mathcal{L}_\theta = \mathbb{E}_{s,a,r,s'} \bigg[\bigg(r + \gamma Q^{target}(s,a; \theta) - Q^{policy}(s,a; \theta) \bigg)^2 \bigg] 
    \label{eq:rl}
\end{equation}

Here, $Q^{target}(s,a; \theta)$ is only used to calculate the target value $r + \gamma Q^{target}(s,a; \theta)$ and $Q^{policy}(s,a; \theta)$ is used to generate new actions. These two networks have the same architecture but different parameters. Every $T$ steps, $Q^{target}(s,a; \theta)$ synchronizes its parameters with $Q^{policy}(s,a; \theta)$. This strategy can help stabilize the learning
procedure and avoid the divergence of parameters. 
Finally, 
\begin{algorithm}[t]
    \SetAlgoLined
	\KwIn{Original training set, synchronize parameter $k$}
	\KwOut{Optimal deep Q-function $Q(s,a)$}
	Initialize replay memory $D$\;
	Initialize $Q^{policy}(s,a)$ and $Q^{target}(s,a)$ with random weights\;
	\For {epochs $=1,\cdots,M$}{
	    Linearly decay the random sampling ratio $\epsilon$\;
	    Sample a batch of controlled users\;
	    \For {epochs $=1,\cdots,M$}{
	        Toss a coin $p\sim Bernoulli(1-\epsilon)$\;
	        \uIf{p=1}
	        {Random sample action $a_t$\;}
	        \Else{
	        Retrieval current state $s_t$ and sample action $a_t$ from the $Q^{policy}$\;
	        }
	        Generate sequential activity samples for controlled users.\;
	        Inject the samples into the outcome estimator and get the reward $r_t$\;
	        Save current experience $(s_t, a_t, r_t, s_{t+1})$ into replay memory $D$\;
	    }
		Sample a batch $(s_t, a_t, r_t, s_{t+1})$ from the replay memory $D$ with balanced rewards \;
		Calculate target values: $r + \gamma Q^{target}(s_t, a_t)$\;
		Update the parameter of $Q^{policy}(s_t, a_t)$ according to Eq.~\eqref{eq:rl}\;
		\If {$mod(epoch, k)=0$}{
		    Synchornize the parameters of $Q^{target}(s_t, a_t)$ with $Q^{policy}(s_t, a_t)$\;
		}
	}
	\caption{Training Algorithm of DQN}
	\label{alg:dqn}
\end{algorithm}
